# Supplementary material for: On the floating of the topological surface state on top of a thick lead layer: The case of the Pb/Bi2Se3 interface
Source: arXiv:2308.13316 source file (2023-11-27)
Supplement: Supplementary file 1 [file SM_PRM_resub_revised_newtitle.pdf]

# Supplemental Material
# "On the floating of the topological surface state on top of a thick lead layer: The case of the Pb/$Bi_2Se_3$ interface"

Oreste De Luca,[1,2] Igor A. Shvets,[3] Sergey V. Eremeev,[4] Ziya S. Aliev,[5] Marek Kopciuszynski,[6] Alexey Barinov,[6] Fabio Ronci,[7] Stefano Colonna,[7] Evgueni V. Chulkov,[8,9,10,11] Raffaele G. Agostino,[1,2] Marco Papagno,[1,2] and Roberto Flammini[7,*]

[1]*Laboratorio di Spettroscopia Avanzata dei Materiali, STAR IR, Via Tito Flavio, Università della Calabria, 87036, Rende (CS), Italy*
[2]*Dipartimento di Fisica, Università della Calabria, Via P.Bucci, 87036 Arcavacata di Rende (CS), Italy*
[3]*Tomsk State University, 634050 Tomsk, Russia*
[4]*Institute of Strength Physics and Materials Science, Russian Academy of Sciences, 634055 Tomsk, Russia*
[5]*Baku State University, AZ1148 Baku, Azerbaijan*
[6]*Sincrotrone Trieste S.C.p.A., Area Science Park, I-34012 Basovizza, Trieste, Italy*
[7]*Istituto di Struttura della Materia-CNR (ISM-CNR), Via del Fosso del Cavaliere, 00133 Roma, Italy*
[8]*Departamento de Polímeros y Materiales Avanzados: Física, Química y Tecnología, Facultad de Ciencias Químicas, Universidad del País Vasco UPV/EHU, 20080 San Sebastián/Donostia, Spain*
[9]*Donostia International Physics Center (DIPC), 20018 Donostia-San Sebastián, Basque Country, Spain*
[10]*Centro de Física de Materiales (CFM-MPC), Centro Mixto CSIC-UPV/EHU, 20018 Donostia-San Sebastián, Basque Country, Spain*
[11]*Saint Petersburg State University, 199034 Saint Petersburg, Russia*

(Dated: November 23, 2023)

## LIST OF SUPPLEMENTAL EXPERIMENTAL AND THEORETICAL DATA

- Dependence of the valence bands and of the loss spectra as a function of the thickness and of the temperature. **Fig.S1** and **Fig.S2**.
- Surface electronic structure of the 1 ML Pb/Bi2Se3 interface with Pb in the fcc-hollow position. **Fig.S3**

* Roberto.Flammini@cnr.it

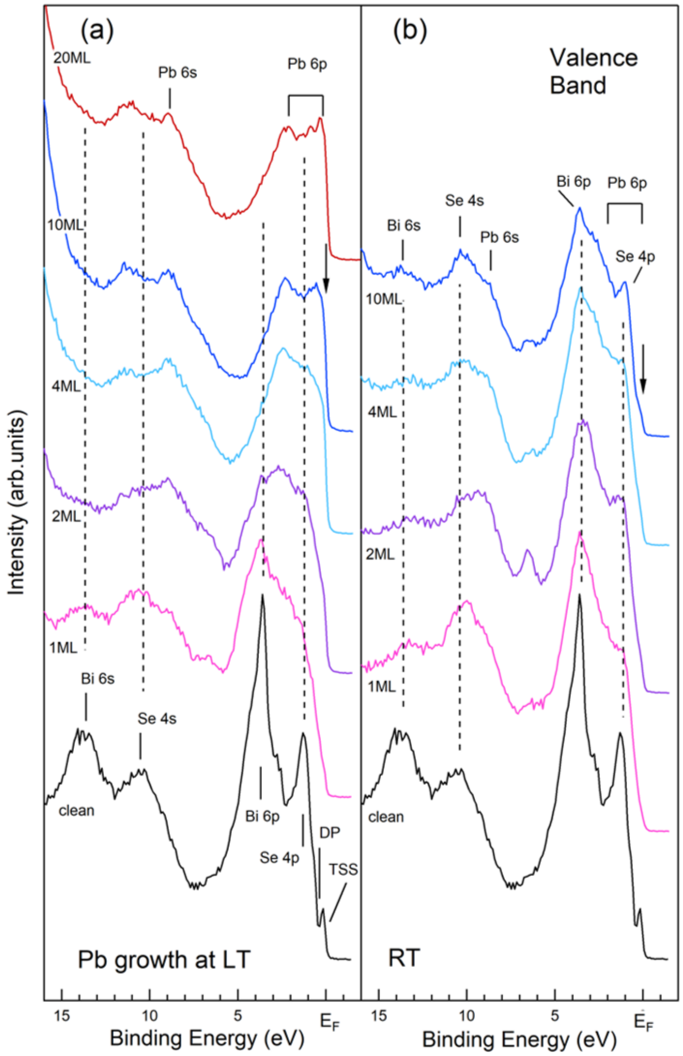


FIG. S1. Valence band spectra taken at $h\nu = 74$ eV photon energy. The color scheme follows that of the main manuscript. Panel (a) features the evolution of the valence bands as a function of the deposit at LN temperature. In panel (b), the spectra taken for the same amount of Pb, after the sample is left to return to RT. The black vertical arrows highlight the change of the density of the states near the Fermi level. DP and TSS stand for Dirac Point and Topological Surface State, respectively.

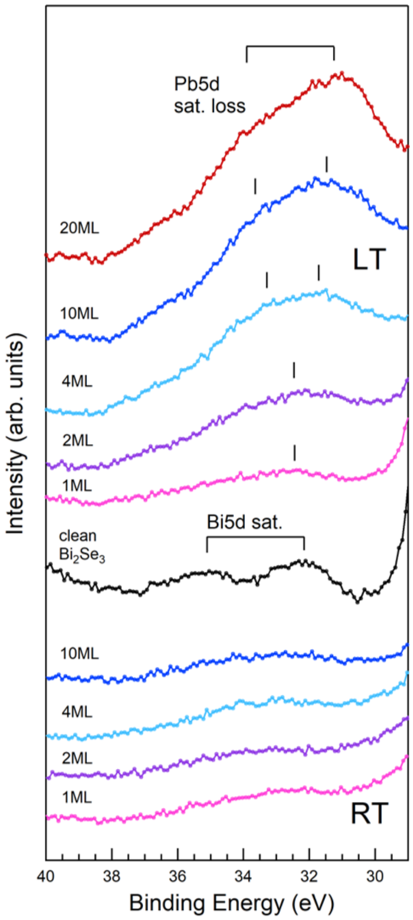


FIG. S2. Photoelectron spectra relative to the energy range of the satellite losses. The photon energy is $h\nu = 74$ eV. The color scheme follows that of the main manuscript. On the top, the spectra taken during the deposit at LN temperature are displayed while, at the bottom, after the sample is left to return to RT.

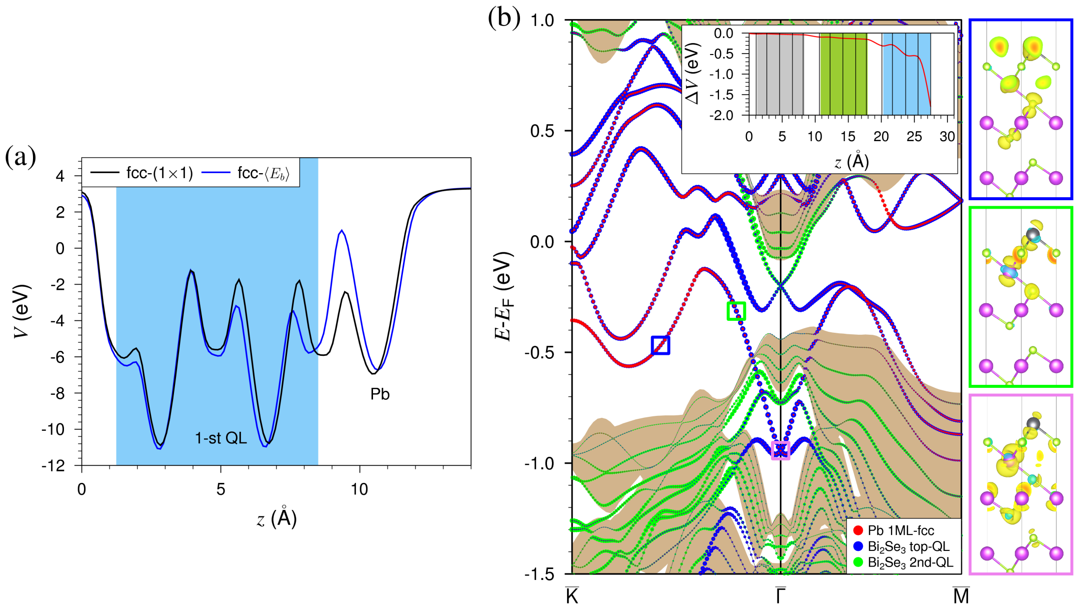


FIG. S3. (a) In-plane averaged electrostatic potentials $V_z$ for $Pb/Bi_2Se_3$ with Pb in fcc position obtained within a $1 \times 1$ relaxed cell (fcc-($1 \times 1$)) and with interatomic distances extracted from the ($6/5 \times 6/5$) model with Pb in fcc-hollow (fcc-$\langle E_b \rangle$). Zero $z$ corresponds to the middle of the first vdW gap. (b) Surface electronic structure of the 1 ML $Pb/Bi_2Se_3$ interface with Pb in the fcc-hollow position; inset shows the potential bending $\Delta V_z$ within the $Bi_2Se_3$ slab ($z = 0$ corresponds to the middle of the third vdW gap). Spatial distributions of the surface states marked with colored squares are shown in right outsets framed with the same colors.
